# Supplementary material for: In-Context Learning with Transformers: Softmax Attention Adapts to Function Lipschitzness
Source: arXiv:2402.11639 source file (2024-05-28)
Supplement: Supplementary file 2 [file Sketch-full.tex]

\section{Sketch of the Proof of Theorem \ref{main:general}}\label{sec:proofoverview}
To highlight the key insights of our analysis, in this section we consider a modification of the softmax attention that exhibits important properties of the original. Note that this approximation is for illustration only; the above results use the original softmax attention -- see Appendices \ref{app:bias}, \ref{app:noise}, \ref{app:full}. For now, consider a function class $\F_L := \{ f: f(\bx) = L \mathbf{w}^\top \bx, \; \mathbf{w}\in \mathbb{S}^{d-1}\}$ of linear functions.
% Suppose further that $\boldsymbol{\Sigma} = \mathbf{I}_d$.

\para{(Temporary) modification of the softmax attention.}
Rather than averaging over every token with a weight that decays exponentially with distance, we consider a modification which \textit{uniformly} averages all tokens within a distance specified by $w_{KQ}=\Vert \mathbf{M}\Vert$. 
% Let $w_{KQ} = \Vert \mathbf{M}\Vert$, then 
From Lemma \ref{lem:assumptionssatisfyidentity}, without loss of generality (WLOG) we can consider $ \mathbf{M} = w_{KQ} \mathbf{I}_d$.
This means that, ignoring normalization, the weight assigned to $f(\bx_i)$ by the true soft-max attention is  $e^{-w_{KQ} \Vert \bx-\bx_i\Vert^2}$. That is, for all $\bx_i$ satisfying $\Vert \bx - \bx_i\Vert < \nicefrac{1}{\sqrt{w_{KQ}}}$, the assigned weights are all $\Theta(1)$, specifically in $(e^{-1},1]$.
% within a constant factor of each other. 
Meanwhile, for $\bx_i$ satisfying $\Vert \bx-\bx_i\Vert = \nicefrac{\sqrt{c}}{\sqrt{w_{KQ}}}$ for $c>1$, the weights are $e^{-c}$, decaying exponentially in $c$. This motivates us to consider a ``modified softmax attention" given by $h_{MSA}(\bx) := \sum_i \frac{f(\bx_i) \mathbbm{1}_i}{\sum_j \mathbbm{1}_j},$
where 
$\mathbbm{1}_j := \mathbbm{1}\{\Vert \bx-\bx_j\Vert < \nicefrac{1}{\sqrt{w_{KQ}}}\}$. In particular, $h_{MSA}(\bx)$  uniformly averages the labels of points within a Euclidean ball of radius $\nicefrac{1}{\sqrt{w_{KQ}}}$ around $\bx$, and ignores all others.

\para{The In-Context Loss.}
Since the (label) noise is independent of all other random variables, the pretraining loss from Equation \ref{eq:loss} can be decomposed into distinct weighted sums of labels and noise:
$$\uL(w_{KQ}\mathbf{I}_d) = \underbrace{\E_{f, \{\bx_i\}_i} \left( \sum_j \frac{(f(\bx_{n+1})- f(\bx_j))\mathbbm{1}_j}{\sum_j \mathbbm{1}_j}\right)^2}_{=:\uLb(w_{KQ})} + \underbrace{\E_{\{\bx_i\}_i, \{\epsilon_i\}_i}  \left(\sum_i \frac{\epsilon_i\mathbbm{1}_i}{\sum_j \mathbbm{1}_j}\right)^2}_{=:\uLn(w_{KQ})}.$$
We first upper and lower bound each of these terms separately, starting with $\uLb(w_{KQ})$.

\para{Noiseless Estimator Bias.} (Please see Appendix \ref{app:bias})
% Suppose the function class $\F$ is Lipschitz, satisfying 
% $$\forall ~ f, \bx, \bx', \hspace{0.2cm}|f(\bx)-f(\bx')|\le L\Vert \bx-\bx'\Vert.$$
% Then we have 
% We begin our analysis of $\uLb(w_{KQ}) $ by upper bounding it using the Lipschitzness of $\mathcal{F}$ (Assumption \ref{main:assumptions}) and the definition of $\mathbbm{1}_j$.
% \begin{align*} 
% \uLb(w_{KQ}) 
% % &= \E_{f, \{\bx_i\}} \left(f(\bx_{n+1}) - \frac{\sum_j f(\bx_j)\mathbbm{1}_j}{\sum_j \mathbbm{1}_j}\right)^2\\
% &\le \E_{f, \{\bx_i\}} \left(\frac{\sum_j L\Vert \bx_{n+1}-\bx_j\Vert \mathbbm{1}_j}{\sum_j \mathbbm{1}_j}\right)^2\le \E_{f, \{\bx_i\}} \left(\frac{\sum_j L\frac{1}{\sqrt{w_{KQ}}} \mathbbm{1}_j}{\sum_j \mathbbm{1}_j}\right)^2 = \frac{L^2}{w_{KQ}}\\
% \end{align*}
% Deriving a meaningful lower bound requires more work. Consider for instance a function class $\mathcal{F}$ consisting of constant functions, i.e. $f(x)=c$. Then $\uLb(w_{KQ}) =0$ for all distributions over $\mathcal{F}$ and all
% $w_{KQ}$. Thus, roughly speaking, to lower bound $\uLb(w_{KQ})$ away from zero we must leverage a lower bound on the complexity of the function class.
This term is the squared difference between an unweighted average of the token labels within a radius of $\bx$, and the true label. Take $w_{KQ} = \Omega(1)$. Then for large $d$, most of the points $\bx_i$ satisfying $\Vert \bx-\bx_i\Vert \le \nicefrac{1}{\sqrt{w_{KQ}}}$ lie on the boundary of the cap, that is, $\Vert \bx - \bx_i\Vert <\nicefrac{1}{\sqrt{w_{KQ}}}\implies \Vert \bx - \bx_i\Vert \approx\nicefrac{1}{\sqrt{w_{KQ}}}.$
This motivates us to approximate the set of points $\bx_i$ satisfying the above as coming from a uniform distribution over just the boundary of the cap. The center of mass of a ring of radius $\nicefrac{1}{\sqrt{w_{KQ}}}$ embedded on the surface of a hyper-sphere, is $\uO(\nicefrac{1}{w_{KQ}})$ from the boundary of a sphere, so the squared bias is $\Theta(\nicefrac{L^2}{w^2_{KQ}})$.
% Denote by $\uU_{\bx, \epsilon}$ the uniform distribution over $\bx'$ such that $\Vert \bx-\bx'\Vert = \epsilon$. Now we have
% \begin{align*} 
% \sum_i\frac{\mathbbm{1}_i f(\bx_i)}{\sum_j \mathbbm{1}_j} &= \sum_i\frac{\mathbbm{1}_i \mathbf{w}^\top \bx_i}{\sum_j \mathbbm{1}_j}\approx \mathbf{w}^\top \E_{\bx'\sim \uU_{\bx, \frac{1}{\sqrt{w_{KQ}}}}} \bx'=\mathbf{w}^\top \left(\E_{\bx'\sim \uU_{\bx, \frac{1}{\sqrt{w_{KQ}}}}} \left(\frac{\bx' + (2\bx\bx^\top -I)\bx'}{2}\right)\right)\\
% & =\mathbf{w}^\top\bx \left(\E_{\bx'\sim \uU_{\bx, \frac{1}{\sqrt{w_{KQ}}}}} \bx^\top\bx'\right)= \mathbf{w}^\top \bx \left(1-\frac{1}{w_{KQ}}\right)
% \end{align*}
% The squared difference is simply
% \begin{align*}
%     \E_{f, \{bx_i\}}\left[\left(f(\bx)-\sum_i\frac{\mathbbm{1}_i f(\bx_i)}{\sum_j \mathbbm{1}_j}\right)^2\right] 
%     &\approx \E_{f, \{bx\}} \left[\left(\mathbf{w}^\top \bx-\mathbf{w}^\top \bx \left(1-\frac{1}{w_{KQ}}\right)\right)^2\right]= \frac{L^2}{dw_{KQ}^2}\\
% \end{align*}

\para{Noise.} (Please see Appendix \ref{app:noise} for details) Since the noise is independent across tokens, expanding the square reveals that  $\mathcal{L}_{\text{noise}}(w_{KQ}) = \frac{\sigma^2}{\sum_j \mathbbm{1}_j}$, which is proportional to  the reciprocal of the number of tokens found within a $\nicefrac{1}{\sqrt{w_{KQ}}}$ radius of $\bx$. In Lemma \ref{lem:capbounds}, we derive bounds for the measure in this region and for now we ignore any finite-sample effects and replace the sum in the denominator with its expectation. This allows us to bound $\frac{1}{\sum_j \mathbbm{1}_j} = \Theta\big(\nicefrac{w_{KQ}^{\frac{d}{2}}}{n}\big)$ as long as $w_{KQ}\lesssim n^{2/d}$. 
% {\color{red} ... we also need something like $w_{KQ}\approx\Theta(1)$ for this to hold, right?}

\para{Combining the $\uLb$ and $\uLn$ terms.} (Please see Appendix \ref{app:full} for details)
Overall, we have $\uL = \uLb + \uLn$ with $\uLb= \Theta\big(\nicefrac{L^2}{w_{KQ}}\big)$ and $\uLn =\Theta\big( \nicefrac{w_{KQ}^{\frac{d}{2}}\sigma^2 }{n}\big)$. Minimizing this sum reveals that the optimal $w_{KQ}$ satisfies $w_{KQ} = \Theta\big((\nicefrac{nL^2}{\sigma^2})^{\frac{2}{d+2}}\big)$.
