# Supplementary material for: In-Context Learning with Transformers: Softmax Attention Adapts to Function Lipschitzness
Source: arXiv:2402.11639 source file (2024-05-28)
Supplement: Supplementary file 3 [file Variance.tex]

\section{Variance}

In this section we control the variance term in the loss.

Given a context $\mathbf{X}_t \in \mathbb{R}^{(d+1)\times (n+1)}$, the prediction of $y_{t,n+1}$ by the one-layer transformer described in Section \ref{sec:formulation} is given by:
\begin{align*}
\hat y_{t,n+1}
&= 
\mathbf{v}_{:d}^\top  \sum_{i=1}^n \mathbf{x}_{t,i} \frac{\exp({\beta \mathbf{x}_{t,i}^\top \bK^\top \bQ \mathbf{x}_{t,n+1}})}{ \sum_{i'=1}^n \exp(\beta \mathbf{x}_{t,i'}^\top \mathbf{K}^\top \mathbf{Q} \mathbf{x}_{t,n+1} )
} 
+ 
{v}_{d+1} \sum_{i=1}^n (f_t(\mathbf{x}_{t,i})+\epsilon_{t,i}) \frac{\exp({\beta \mathbf{x}_{t,i}^\top \bK^\top \bQ \mathbf{x}_{t,n+1}})}{
\sum_{i'=1}^n \exp(\beta \mathbf{x}_{t,i'}^\top \mathbf{K}^\top \mathbf{Q} \mathbf{x}_{t,n+1} )
} \nonumber 
\end{align*}
% where we define $v\mathbf{w}_t := \mathbf{v}_{:d} + v_{d+1} \mathbf{w}_{\ast,t}$ and
In the following we denote  $\mathbf{M} \coloneqq \beta \mathbf{K}^\top \mathbf{Q}$ and drop subscripts $t$ indicating the context for ease of notation. 
{
We also let
$\hat{\mathbf{x}}_{n+1}  \coloneqq \sum_{i=1}^n \mathbf{x}_{i} \frac{\exp({\mathbf{x}_{i}^\top \mathbf{M} \mathbf{x}_{n+1}})}{ \sum_{i'=1}^n \exp( \mathbf{x}_{i'}^\top \mathbf{M} \mathbf{x}_{n+1} )
}  $, 
$\hat{f}_t(x_{n+1})  \coloneqq \sum_{i=1}^n f_t(x_i) \frac{\exp({\mathbf{x}_{i}^\top \mathbf{M} \mathbf{x}_{n+1}})}{ \sum_{i'=1}^n \exp( \mathbf{x}_{i'}^\top \mathbf{M} \mathbf{x}_{n+1} )
}  $, and 
$\hat{\epsilon} \coloneqq \sum_{i=1}^n \epsilon_{i} \frac{\exp({\mathbf{x}_{i}^\top \mathbf{M} \mathbf{x}_{n+1}})}{ \sum_{i'=1}^n \exp( \mathbf{x}_{i'}^\top \mathbf{M} \mathbf{x}_{n+1} )
} $.

}

Using this notation, we have $\hat{y}_{n+1} = \mathbf{v}_{:d}^\top \hat{\mathbf{x}}_{n+1} + v_{d+1}\hat{f}_t(x_{n+1}) + v_{d+1} \hat{\epsilon} $, and the 
% the transformer prediction can be written as $\hat{y}_{n+1}= v\mathbf{w}_t^\top  \sum_{i=1}^n \mathbf{x}_{i} \alpha_{i}(\{\mathbf{x}_i\}_{i\in[n]})  + v_{d+1}\sum_{i=1}^n \epsilon_{i} \alpha_{i}(\{\mathbf{x}_i\}_{i\in[n]})$, and  
training population loss over the distribution of contexts is given by:
\begin{align}
\mathcal{L}(\mathbf{M},\mathbf{v}) &:= \tfrac{1}{2}\E_{\mathbf{w},\{\mathbf{x}_{i}\}_{i},\{\epsilon_i\}_i} \left[(\hat y_{n+1}-\mathbf{w}^\top \mathbf{x}_{n+1})^2\right] \label{pop}\\
&= \tfrac{1}{2}\E_{\mathbf{w},\{\mathbf{x}_{i}\}_{i},\{\epsilon_i\}_i} \left[(\mathbf{w}^\top (v_{d+1}\hat{\mathbf{x}}_{n+1}-\mathbf{x}_{n+1}) + \mathbf{v}_{:d}^\top \hat{\mathbf{x}}_{n+1} + v_{d+1}\hat{\epsilon} )^2\right] \nonumber \\
&= \tfrac{1}{2}\E_{\mathbf{w},\{\mathbf{x}_{i}\}_{i},\{\epsilon_i\}_i} \left[(\mathbf{w}^\top (v_{d+1}\hat{\mathbf{x}}_{n+1}-\mathbf{x}_{n+1}) + v_{d+1}\hat{\epsilon} )^2\right] +\tfrac{1}{2}\E_{\{\mathbf{x}_{i}\}_i} \left[ (\mathbf{v}_{:d}^\top \hat{\mathbf{x}}_{n+1})^2 \right] \nonumber \\
&\quad + \E_{\mathbf{w},\{\mathbf{x}_{i}\}_{i},\{\epsilon_i\}_i} \left[  \mathbf{v}_{:d}^\top \hat{\mathbf{x}}_{n+1}  (\mathbf{w}^\top (v_{d+1}\hat{\mathbf{x}}_{n+1}-\mathbf{x}_{n+1}) + v_{d+1}\hat{\epsilon} )\right] \nonumber \\
&\stackrel{a}{=} \tfrac{1}{2}\E_{\mathbf{w},\{\mathbf{x}_{i}\}_{i},\{\epsilon_i\}_i} \left[(\mathbf{w}^\top (v_{d+1}\hat{\mathbf{x}}_{n+1}-\mathbf{x}_{n+1}) + v_{d+1}\hat{\epsilon} )^2\right] +\tfrac{1}{2}\E_{\{\mathbf{x}_{i}\}_i} \left[ (\mathbf{v}_{:d}^\top \hat{\mathbf{x}}_{n+1})^2 \right] \nonumber \\
&\stackrel{b}{\geq} \tfrac{1}{2}\E_{f_t,\{\mathbf{x}_{i}\}_{i},\{\epsilon_i\}_i} \left[(v_{d+1}\hat{f}_t(x_{n+1})-f_t({x}_{n+1}) + v_{d+1}\hat{\epsilon} )^2\right] \label{3}
\end{align}
where $a$ follows by the fact that  $\mathbf{w}$ and each $\epsilon_i$ are zero-mean and independent of all other quantities, and $b$ follows since $ (\mathbf{v}_{:d}^\top \hat{\mathbf{x}}_{n+1})^2 \geq 0$. Moreover, $\E_{\{\mathbf{x}_{i}\}_i} \left[ (\mathbf{v}_{:d}^\top \hat{\mathbf{x}}_{n+1})^2 \right]=0 \iff \mathbf{v}_{:d}=\mathbf{0}_d$. So, any global minimizer $(\mathbf{M}^*, \mathbf{v}^*)$ of $\mathcal{L}$ must satisfy $\mathbf{v}^*_{:d}= \mathbf{0}_d$. Therefore we set $\mathbf{v}_{:d} = \mathbf{0}_d$ in all subsequent analysis, and consider the loss from \eqref{3}: $$
\tilde{\mathcal{L}}(\mathbf{M},v) := \tfrac{1}{2}\E_{\mathbf{w},\{\mathbf{x}_{i}\}_{i},\{\epsilon_i\}_i} \left[(\mathbf{w}^\top (v\hat{\mathbf{x}}_{n+1}-\mathbf{x}_{n+1}) + v\hat{\epsilon} )^2\right], 
$$
where we have replaced $v_{d+1}$ with $v$ for ease of notation.
Next, expanding the square yields
\begin{align}
    \tilde{\mathcal{L}}(\mathbf{M},v)  &= \tfrac{1}{2}\E_{f_t,\{\mathbf{x}_{i}\}_{i}} \left[(v_{d+1}\hat{f}_t(x_{n+1})-f_t({x}_{n+1}))^2\right]  + \tfrac{1}{2}\E_{\{\mathbf{x}_{i}\}_{i},\{\epsilon_i\}_i} \left[ v^2\hat{\epsilon}^2\right],
\end{align}
since each noise $\epsilon_i$ is mean-zero and independent of all other terms.

For ease of exposition, we assume $v=1$ in the following. We have
\begin{align}
    \tilde{\mathcal{L}}(\mathbf{M})  &= \tfrac{1}{2}\E_{f_t,x_{n+1}} \left[(\mathbb{E}_{x_i}[\hat{f}_t(x_{n+1})]-f_t({x}_{n+1}))^2\right] + \tfrac{1}{2}\E_{f_t,\{x_i\}_i,x_{n+1}} \left[(\hat{f}_t({x}_{n+1})-\mathbb{E}_{x_i}[\hat{f}_t(x_{n+1})])^2\right]  + \tfrac{1}{2}\E_{\{\mathbf{x}_{i}\}_{i},\{\epsilon_i\}_i} \left[ v^2\hat{\epsilon}^2\right],
\end{align}

% \begin{align}
% \tilde{\mathcal{L}}(\mathbf{M},v)  &= 
% \tfrac{1}{2}\E_{\mathbf{w}_\ast,\{\mathbf{x}_{i}\}_{i},\{\epsilon_i\}_i} \left[\left( v\mathbf{w}^\top   \frac{\sum_{i=1}^n \mathbf{x}_{i}\exp({\mathbf{x}_{i}^\top \mathbf{M} \mathbf{x}_{n+1}})}{ \sum_{i=1}^n \exp(\mathbf{x}_{i}^\top \mathbf{M} \mathbf{x}_{n+1} )
% }  + v_{d+1}\frac{\sum_{i=1}^n \epsilon_{i} \exp({\mathbf{x}_{i}^\top \mathbf{M} \mathbf{x}_{n+1}})}{ \sum_{i=1}^n \exp(\mathbf{x}_{i}^\top \mathbf{M} \mathbf{x}_{n+1} )}
% - \mathbf{w}_{\ast}^\top \mathbf{x}_{n+1}\right)^2 \right] \nonumber \\
% &= \tfrac{1}{2}\E_{\mathbf{w}_\ast,\{\mathbf{x}_{i}\}_{i}} \Bigg[\left( v\mathbf{w}^\top   \frac{\sum_{i=1}^n \mathbf{x}_{i}\exp({\mathbf{x}_{i}^\top \mathbf{M} \mathbf{x}_{n+1}})}{ \sum_{i=1}^n \exp(\mathbf{x}_{i}^\top \mathbf{M} \mathbf{x}_{n+1} )
% } 
% - \mathbf{w}_{\ast}^\top \mathbf{x}_{n+1}\right)^2 \Bigg]  \nonumber \\
% &\quad + \tfrac{1}{2}\E_{\mathbf{w}_\ast,\{\mathbf{x}_{i}\}_{i},\{\epsilon_i\}_i} \Bigg[\left( v_{d+1}\frac{\sum_{i=1}^n \epsilon_{i} \exp({\mathbf{x}_{i}^\top \mathbf{M} \mathbf{x}_{n+1}})}{ \sum_{i=1}^n \exp(\mathbf{x}_{i}^\top \mathbf{M} \mathbf{x}_{n+1} )}
% \right)^2 \Bigg] 
% \label{noise} 
% \end{align}
% where \eqref{noise} follows since the noise $\epsilon_i$ is mean-zero and independent of all other terms. 

We have 
\begin{align}
    \mathcal{L}_{\text{var}}(M) &= \mathbb{E}_{\{x_i\}_{i=1}^n, x, f_t}\left[\left(\frac{\sum_{i=1}^n (f_t(x_i) - \hat{f}_t(x)) e^{x_i^\top M x }  }{\sum_{i=1}^n e^{x_i^\top M x } }\right)^2 \right] \nonumber \\
    &= n\mathbb{E}_{\{x_i\}_{i=1}^n, x, f_t}\left[\frac{(f_t(x_1) - \hat{f}_t(x))^2 e^{2x_1^\top M x }  }{(\sum_{i=1}^n e^{x_i^\top M x } )^2} \right] + n(n-1)\mathbb{E}_{\{x_i\}_{i=1}^n, x, f_t}\left[\frac{(f_t(x_1) - \hat{f}_t(x))(f_t(x_2) - \hat{f}_t(x))  e^{x_1^\top M x + x_2^\top M x }  }{(\sum_{i=1}^n e^{x_i^\top M x } )^2} \right] 
\end{align}

% We consider the second term.

\begin{align}
    &\mathbb{E}_{\{x_i\}_{i=1}^n, x, f_t}\left[\frac{(\sum_{i=1}^n(f_t(x_i) - \hat{f}_t(x)) e^{x_i^\top M x } )^2 }{(\sum_{i=1}^n e^{x_i^\top M x } )^2} \right] \nonumber \\
    &= \frac{\mathbb{E}_{\{x_i\}_{i=1}^n, x, f_t}\left[(\sum_{i=1}^n(f_t(x_i) - \hat{f}_t(x)) e^{x_i^\top M x  })^2 \right] }{\mathbb{E}_{\{x_i\}_i}[(\sum_{i=1}^n e^{x_i^\top M x } )^2]}\nonumber \\
    &\quad \quad + \left(\mathbb{E}_{\{x_i\}_{i=1}^n, x, f_t}\left[\frac{(\sum_{i=1}^n(f_t(x_i) - \hat{f}_t(x)) e^{x_i^\top M x } )^2 }{(\sum_{i=1}^n e^{x_i^\top M x } )^2} \right] - \frac{\mathbb{E}_{\{x_i\}_{i=1}^n, x, f_t}\left[(\sum_{i=1}^n(f_t(x_i) - \hat{f}_t(x))  e^{x_i^\top M x } )^2 \right] }{\mathbb{E}_{\{x_i\}_i}[(\sum_{i=1}^n e^{x_i^\top M x } )^2]} \right)  \nonumber \\
\end{align}
By a Taylor series expansion of $f(x) \coloneqq 1/x$ around $\mathbb{E}[()^2]$, we have that the error term is:
\begin{align}
    &\mathbb{E}_{\{x_i\}_{i=1}^n, x, f_t}\left[\frac{(\sum_{i=1}^n(f_t(x_i) - \hat{f}_t(x)) e^{x_i^\top M x } )^2 }{(\sum_{i=1}^n e^{x_i^\top M x } )^2} \right] - \frac{\mathbb{E}_{\{x_i\}_{i=1}^n, x, f_t}\left[(\sum_{i=1}^n(f_t(x_i) - \hat{f}_t(x))  e^{x_i^\top M x } )^2 \right] }{\mathbb{E}_{\{x_i\}_i}[(\sum_{i=1}^n e^{x_i^\top M x } )^2]} \nonumber \\
    &= \sum_{k=1}^\infty \frac{(-1)^k}{k!}  \frac{\mathbb{E}_{\{x_i\}_{i=1}^n, x, f_t}\left[(\sum_{i=1}^n(f_t(x_i) - \hat{f}_t(x))  e^{x_i^\top M x } )^2 \left( (\sum_{i=1}^n e^{x_i^\top M x } )^2 -\mathbb{E}_{\{x_i\}_i}[(\sum_{i=1}^n e^{x_i^\top M x } )^2] \right)^k \right] }{\mathbb{E}_{\{x_i\}_i}[(\sum_{i=1}^n e^{x_i^\top M x } )^2]^{k+1}}  \nonumber  
\end{align}
For

Case 1a: full rank, $x_i$ uniform on unit sphere, general phi. Goal: just get uniform upper bound.

% Case 1b: low rank, $x_i$ uniform on unit sphere, general phi. Goal: show variance is regularizer+small, regularizer kills perp part. Problem: we can;t fully characterize opt soln because bias is a function of perp part and can decrease with more perp part.

% in these cases, don't need upper bound on M.

% Case 2: $x_i$ is Gaussian, $f_t$ is linear. case 2a: non-isotropic.
  % case 2b: low rank. 

Later: gaussian data, linear, make denom approx before decomposing loss and say that error is negligible, and scale noise with n. then get low rank and inverse covariance result.

could also do this with normalized data and general phi? normalized and linear? probelm is we

  % to say anything about low-rank, for any data, need to analyze bias+variance together, or make denom approx and say that error is negligible, and scale noise with n.

% need upper bound on M i think, maybe not
