# Supplementary material for: In-Context Learning with Transformers: Softmax Attention Adapts to Function Lipschitzness
Source: arXiv:2402.11639 source file (2024-05-28)
Supplement: Supplementary file 4 [file Lipschitz.tex]

\begin{comment}
\section{Full Rank}

% \begin{assumption}\label{assump:rotation}
%     For any $x,x'\in \mathbb{S}^{d-1}$ and any rotation matrix $\mathbf{R}\in \mathcal{O}^{d\times d}$ (i.e. a matrix satisfying $\mathbf{R}^T\mathbf{R} = \mathbf{RR}^\top = \mathbf{I}_d$), the following holds:
%     \begin{align*}
%         \mathbb{E}_{\phi}[\phi(x)\phi(x')] =  \mathbb{E}_{\phi}[\phi(\mathbf{R}x)\phi(\mathbf{R}x')].
%     \end{align*}
% \end{assumption}
% Assumption \ref{assump:rotation} entails that the correlation between $\phi(x)$ and $\phi(x')$  (with randomness due to choice of $\phi$) is invariant to identical rotations of $x$ and $x'$, in other words, the distribution of $\phi$ is in some sense spherically symmetric about the origin.

% \begin{assumption}\label{assump:corr}
% For any $c > 0$, define $\mu_c(\phi, x) \coloneqq \mathbb{E}_{x_1,\dots,x_n \stackrel{\text{iid}}{\sim} \text{Unif}(\mathbb{S}^{d-1})}\left[\frac{\phi(x_1)e^{c x_1^\top x}}{\sum_{i=1}^n e^{c x_i^\top x} }\right]$.
% For any $x,x'\in \mathbb{S}^{d-1}$ such that $x \neq x'$, 
% \begin{align*}
%     \mathbb{E}_{\phi}[\mu_c(\phi,x)\phi(x)] >  \mathbb{E}_{\phi}[\mu_c(\phi,x)\phi(x')].
% \end{align*}
% \end{assumption}

% Assumption \ref{assump:corr} states that $\mu_c(\phi,x)$ is more correlated with $\phi(x)$ than $\phi(x')$ for any $x'\neq x$, where the randomness is due to the choice of $\phi$. Note that $\mu_c(\phi,x)$ is a weighted average of  $\phi(x_1)$ across $x_1$ on the unit hypersphere, where the weights scale exponentially with $x_1^T x$, so  $\mu_c(\phi,x)$ can be thought of as a prediction of $\phi(x)$, so it is natural to assume that $\mu_c(\phi,x)$ is more correlated with $\phi(x)$ than $\phi(x')$ for any other $x'$.

We first prove that under Assumptions \ref{assump:rotation} and \ref{assump:corr}, the optimal $W_k^\top W_Q$ is a scalar times identity.
\begin{lemma}\label{lemma:identityM}
    Under Assumptions \ref{assump:rotation} and \ref{assump:corr}, the optimal $W_Q, W_K$ for $\uL$ defined as in \ref{eq:loss} satisfy $W_Q^\top W_K = c^*I$ for some scalar $c^*$.
\end{lemma}

\begin{proof}
 We denote $M =W_K^T W_Q $ and $x=x_{n+1}$ for ease of notation. 
The first step in the proof entails writing the loss of $M$ as the expectation over $x$ of the loss of $M$ on  $x$. Then, we decompose the action of $M$ on $x$  into a rotation and a scaling, such that the rotation does not appear in any exponent in the loss. This will allow us to compare the loss to the analogous loss with rotation set to identity, and show that the latter loss is smaller, which implies that any optimal $M$ for $x$ must be such that $Mx$ is parallel $x$. Finally, we show that there exists some $M^*$ that achieves this minimum value for all $x\in \mathbb{S}^{d-1}$; in particular, this $M^*$ satisfies $M^*=c^*I$ for some  nonzero scalar $c^*$. Moreover, any $M$ that is not a scaled identity achieves strictly larger loss.


% i.e., any optimal $M$ must be a scalar times identity.

\vspace{2mm}

To this end, first recall the population loss defined in \eqref{}. For ease of notation, we use $\mathbb{E}_{f, x, \{x_i\}_{i=1}^n}$ to denote $\mathbb{E}_{f \sim D(\mathcal{F}), x \sim \mathcal{U}^d, \{x_i\}_{i=1}^n \stackrel{\text{i.i.d.}}{\sim} \mathcal{U}^{d \times n} }$. 
\begin{align}
  \mathcal{L}(M) &=   \mathbb{E}_{f, x, \{x_i\}_{i=1}^n} \left[\left( \frac{\sum_{i=1}^n(f(x_i) - f(x) + \epsilon_i )e^{x_i^\top Mx  } }{\sum_{i=1}^n e^{x_i^\top M x}}  \right)^2 \right] \nonumber 
  \end{align}
  We move the expectation over $x$ to the outside and write
  \begin{align}
      \mathcal{L}(M) &=   \mathbb{E}_{x} \left[\mathcal{L}(M;x)\right] \nonumber 
  \end{align}
  where 
  \begin{align}
      \mathcal{L}(M;x) := \mathbb{E}_{f, \{x_i\}_{i=1}^n} \left[\left( \frac{\sum_{i=1}^n(f(x_i) - f(x) + \epsilon_i )e^{x_i^\top Mx  } }{\sum_{i=1}^n e^{x_i^\top M x}}  \right)^2 \right]\label{lohs}
  \end{align}
  is the loss of $M$ on some fixed $x\in \mathbb{S}^{d-1}$. 

\vspace{2mm}

Next we decompose $Mx$ into a rotation and a scaling.
 Note that for any $x\in \mathbb{S}^{d-1}$, 
$M x = R x \|{M}x\|_2$ for some rotation matrix $R \in \mathbb{O}^{d\times d}$ without loss of generality.
Making this substitution in the loss on $x$ in \eqref{lohs} allows us to rewrite this loss as:
\begin{align}
  \mathcal{L}(M;x) &=   \mathbb{E}_{f,  \{x_i\}_{i=1}^n} \left[\left( \frac{\sum_{i=1}^n(f(x_i) - f(x) + \epsilon_i )e^{x_i^\top R x \|{M}x\|_2 } }{\sum_{i=1}^n e^{x_i^\top R x \|{M}x\|_2}}  \right)^2 \right] \nonumber \\
  &=   \mathbb{E}_{  \{x_i\}_{i=1}^n} \left[  \frac{ \mathbb{E}_f[ (f(x_1) - f(x) )^2 ] e^{2 x_1^\top R x \|{M}x\|_2 } }{\left(\sum_{i=1}^n e^{x_i^\top R x \|{M}x\|_2} \right)^2 }   \right] \nonumber \\
  &\quad + \mathbb{E}_{\{x_i\}_{i=1}^n} \left[  \frac{ \mathbb{E}_f [ (f(x_1) - f(x) )  (f(x_2) - f(x) ) ]  e^{x_1^\top R x \|{M}x\|_2  + x_2^\top R x \|{M}x\|_2 } }{\left(\sum_{i=1}^n e^{x_i^\top  R x \|{M}x\|_2} \right)^2 }   \right]  \nonumber \\
  &\quad +    \sigma^2  \mathbb{E}_{f,  \{x_i\}_{i=1}^n} \left[ \frac{  e^{ 2 x_1^\top R x \|{M}x\|_2 } }{ (\sum_{i=1}^n e^{x_i^\top R x \|{M}x\|_2})^2  }   \right]  \nonumber \\
&=  n\mathbb{E}_{ \{x_i\}_{i=1}^n} \left[  \frac{ \mathbb{E}_f[ (f(R^\top x_1) - f(R^\top x) )^2 ] e^{2 x_1^\top R x \|{M}x\|_2 } }{(\sum_{i=1}^n e^{x_i^\top R x \|{M}x\|_2} )^2 }   \right] \nonumber \\
&\quad + n(n-1) \mathbb{E}_{ \{x_i\}_{i=1}^n} \Bigg[   \mathbb{E}_f [ (f( R^\top x_1) - f(R^\top x) )  (f(R^\top x_2) - f(R^\top x) ) ]    \nonumber \\
&\quad  \quad \quad \quad \quad \quad \quad \quad \quad \quad \quad \times \frac{ e^{x_1^\top R x \|{M}x\|_2  + x_2^\top R x \|{M}x\|_2 } }{(\sum_{i=1}^n e^{x_i^\top R x \|{M}x\|_2} )^2 }   \Bigg]  \nonumber \\
&\quad +    \sigma^2  \mathbb{E}_{  \{x_i\}_{i=1}^n} \left[ \frac{  e^{ 2 x_1^\top R x \|{M}x\|_2 } }{ (\sum_{i=1}^n e^{x_i^\top R x \|{M}x\|_2})^2  }   \right]  \label{rot1} \\
&=  n\mathbb{E}_{  \{x_i\}_{i=1}^n} \left[  \frac{ \mathbb{E}_f[ (f(x_1) - f(R^\top x) )^2 ] e^{2 x_1^\top x \|{M}x\|_2 } }{\left(\sum_{i=1}^n e^{x_i^\top x \|{M}x\|_2} \right)^2 }   \right] \nonumber \\
&\quad + n(n-1)\mathbb{E}_{\{x_i\}_{i=1}^n} \Bigg[ \mathbb{E}_f [ (f(  x_1) - f(R^\top x) )  (f( x_2) - f(R^\top x) ) ]     \nonumber \\
&\quad \quad \quad \quad \quad \quad \quad \quad \quad \quad \quad \times  \frac{ e^{x_1^\top x \|{M}x\|_2  + x_2^\top x \|{M}x\|_2}  }{(\sum_{i=1}^n e^{x_i^\top x \|{M}x\|_2} )^2 }   \Bigg] \nonumber \\
&\quad +    \sigma^2  \mathbb{E}_{  \{x_i\}_{i=1}^n} \left[ \frac{  e^{ 2 x_1^\top x \|{M}x\|_2 } }{ \left(\sum_{i=1}^n e^{x_i^\top x \|{M}x\|_2}\right)^2  }   \right]  \label{rot2}
\end{align}
where \eqref{rot1} follows by Assumption \ref{assump:rotation} and \eqref{rot2} follows since the distribution of each $x_i$ is rotation-invariant.
Denote the RHS of \eqref{rot2} by $g(R)$. We next show that $g(R) - g(I) > 0$ for any $R \neq I$.
\begin{align}
&g(R) - g(I)\nonumber \\
&= n\mathbb{E}_{ \{x_i\}_{i=1}^n} \left[  \frac{ \mathbb{E}_f[ (f(x_1) - f(R^\top x) )^2 - (f(x_1) - f(x) )^2  ] e^{2 x_1^\top x \|{M}x\|_2 } }{\left(\sum_{i=1}^n e^{x_i^\top x \|{M}x\|_2} \right)^2 }   \right] \nonumber \\
&\quad + n(n-1)\mathbb{E}_{ \{x_i\}_{i=1}^n} \left[  \frac{ \mathbb{E}_f [ (f(  x_1) - f(R^\top x) )  (f( x_2) - f(R^\top x) )  ]  e^{x_1^\top x \|{M}x\|_2  + x_2^\top x \|{M}x\|_2 }}{\left(\sum_{i=1}^n e^{x_i^\top x \|{M}x\|_2} \right)^2 }   \right]    \nonumber \\
&\quad - n(n-1)\mathbb{E}_{ \{x_i\}_{i=1}^n} \left[  \frac{ \mathbb{E}_f [ (f(  x_1) - f( x) )  (f( x_2) - f( x) ) ]  e^{x_1^\top x \|{M}x\|_2  + x_2^\top x \|{M}x\|_2 }}{\left(\sum_{i=1}^n e^{x_i^\top x \|{M}x\|_2} \right)^2 }   \right]    \nonumber \\
&= 2n\mathbb{E}_{ \{x_i\}_{i=1}^n} \left[  \frac{ \mathbb{E}_f[ (f(x_1) f(x)  -f(x_1) f(R^\top x) ) ] e^{2 x_1^\top x \|{M}x\|_2 } }{\left(\sum_{i=1}^n e^{x_i^\top x \|{M}x\|_2} \right)^2 }   \right]  \nonumber \\
&\quad +  n(n-1)\mathbb{E}_{ \{x_i\}_{i=1}^n} \Bigg[ \mathbb{E}_f \left[  f(  x_1) f( x) + f( x_2)  f( x)  -  f(  x_1) f(R^\top x) - f( x_2)  f(R^\top x)  \right]    \nonumber \\
&\quad \quad \quad \quad \quad \quad \quad \quad \quad \quad \quad \times  \frac{   e^{x_1^\top x \|{M}x\|_2  + x_2^\top x \|{M}x\|_2 }}{(\sum_{i=1}^n e^{x_i^\top x \|{M}x\|_2})^2 }   \Bigg]  \nonumber \\
&= 2n\mathbb{E}_{ f,  \{x_i\}_{i=1}^n} \left[  \frac{ (f(x_1) f(x)  -f(x_1) f(R^\top x) )  e^{2 x_1^\top x \|{M}x\|_2 } }{\left(\sum_{i=1}^n e^{x_i^\top x \|{M}x\|_2} \right)^2 }   \right]  \nonumber \\
&\quad +  n(n-1)\mathbb{E}_{f,  \{x_i\}_{i=1}^n} \Bigg[   \left(f(  x_1) f( x) + f( x_2) - f( x)  -  f(  x_1) f(R^\top x) - f( x_2) f(R^\top x) \right)    \nonumber \\
&\quad \quad \quad \quad \quad \quad \quad \quad \quad \quad \quad \times \frac{   e^{x_1^\top x \|{M}x\|_2  + x_2^\top x \|{M}x\|_2 } }{(\sum_{i=1}^n e^{x_i^\top x \|{M}x\|_2} )^2 }   \Bigg]  \nonumber \\
&= 2n \mathbb{E}_{ f,  \{x_i\}_{i=1}^n} \left[ \left(f(x_1) f(x)  -f(x_1) f(R^\top x) \right) e^{ x_1^\top x \|{M}x\|_2 } \frac{ e^{x_1^\top x \|{M}x\|_2 } + (n-1)  e^{x_2^\top x \|{M}x\|_2 } }{\left(\sum_{i=1}^n e^{x_i^\top x \|{M}x\|_2} \right)^2 }   \right]  \label{aa} \\
&=  2n \mathbb{E}_{ f, \{x_i\}_{i=1}^n} \left[ \left(f(x_1) f(x)  -f(x_1) f(R^\top x) \right) e^{x_1^\top x \|Mx\|_2 } \frac{ \sum_{i=1}^n e^{x_i^\top x \|{M}x\|_2 } }{\left(\sum_{i=1}^n e^{x_i^\top x \|{M}x\|_2} \right)^2 }   \right]  \label{bb} \\
&= 2n \mathbb{E}_{ f,  \{x_i\}_{i=1}^n} \left[ \left(f(x_1) f(x)  -f(x_1) f(R^\top x) \right) \frac{ e^{x_1^\top x \|Mx\|_2 }  }{\sum_{i=1}^n e^{x_i^\top x \|{M}x\|_2}  }   \right]  \nonumber \\
&> 0 \label{cor1}
\end{align}
where \eqref{aa} and \eqref{bb} follow by the i.i.d.-ness of the $x_i$’s and \eqref{cor1} follows by Assumption \ref{assump:corr}, with $x’=R^\top x \neq x$.

\vspace{2mm}


% Lemma: E (f - f’)^2 = E (fR - f’R))^2 from assumption rot, easy
% Lemma: c* doesn’t vary with x easy
Therefore, from \eqref{cor1}, we know that for any fixed $x$, $\mathcal{L}(M;x)$ is minimized by an $M$ that does not rotate $x$. However, it is not yet clear whether there exists an $M$ that can simultaneously minimize $\mathcal{L}(M;x) $ for all $x\in \mathbb{S}^{d-1}$.

To show this, for some $x \in \mathbb{S}^{d-1}$, define $$c^* \in \arg \min_{c\in \mathbb{R}} \left\{ \mathcal{L}(cI; x)=  \mathbb{E}_{f,\{x_i\}_{i=1}^n}  \left[\left( \frac{\sum_{i=1}^n(f(x_i) - f(x) + \epsilon_i )e^{c x_i^\top x } }{\sum_{i=1}^n e^{c x_i^\top  x}}  \right)^2 \right]\right\}  .  $$
Note that by the rotational symmetry of the $x_i$’s, $c^*$ minimizes $\mathcal{L}(cI; x)$ for all $x \in \mathbb{S}^{d-1}$. Also, since we have reduced the problem of minimizing $\mathcal{L}(M;x)$ to finding an appropriate scaling of $x$ by \eqref{cor1}, we have that $M^*=c^*I$ minimizes $\mathcal{L}(M;x)$, for all $x\in \mathbb{S}^{d-1}$, so $M^*=c^*I$ must be a minimizer of the full loss $\mathcal{L}(M)$. Further, by \eqref{cor1}, any $M$ that rotates any $x \in \mathbb{S}^{d-1}$ achieves larger loss than $M^*=c^*I$, so any minimizer of $\mathcal{L}(M)$ must be a scaled identity (otherwise it would rotate some $x$).
\end{proof}








% c* unique?

\end{comment}
