# Supplementary material for: In-Context Learning with Transformers: Softmax Attention Adapts to Function Lipschitzness
Source: arXiv:2402.11639 source file (2024-05-28)
Supplement: Supplementary file 5 [file Low-rank-quadratic.tex]

% \subsection{Quadratic Functions}

% In this section we prove Theorem \ref{thm:lin_low_rank}(b), i.e. the case in which the task functions are quadratic. 
% % In particular, we consider the function class

% We state Theorem \ref{thm:lin_low_rank}(b) in full detail here.
% \begin{theorem}\label{thm:app-low-rank-quad}
%     Consider the function class 
%     \begin{align}
%     \mathcal{F}_2 \coloneqq \{ f_w: f_w(x) = (w^\top x), w \in \mathbb{R}^d \}
% \end{align}
% and any distribution $\mathcal{D}$ over $\mathcal{F}_2$ that satisfies $\mathbb{E}[ww^\top] = c_w BB^T$ for some nonzero constant $c_w$.

% Then 
% \end{theorem}


% \begin{proof}
%     We use the same proof technique as in the proof of Theorem \ref{thm_app:lin_low_rank}. 

% Define $U_{\perp} = I - uu^\top$.



% By Lemma \ref{lem:exp-w-quad}, we have 
% \begin{align}
%     \mathbb{E}_w \left[ \left((u_1 -)^\top ww^\top () \right)^2\right] = 2 ()^2 - 1
% \end{align}



% By Lemma \ref{lem:orthog}



    
% Next, as in the proof of Theorem \ref{thm_app:lin_low_rank}, we show that the sum $S_{i,1}+S_{i,i}$ is positive. We have
% \begin{align}
%     s_{i,1}+ s_{i,i} &= (u_1+u_i-2u)^\top (u_1-u) (u_1 - u_i)^\top (u_1-u)\nonumber \\
%     &\quad + (u_1+u_i-2u)^\top (u_i-u) (u_1 - u_i)^\top (u_i-u) \nonumber \\
%     &= (3 + u_1^\top u_i - 3 u_1^\top u - u_i^\top )( 1 - u_1^\top u_i - u_1^\top u + u_i^\top)\nonumber \\
%     &\quad + (3 + u_1^\top u_i - 3 u_i^\top u - u_1^\top )( -1 + u_1^\top u_i - u_1^\top u + u_i^\top)
% \end{align}
% Let $t_1 = $, $t_2 = $, $q_1 = 1- u_1^\top u_i $, and $q_2= $. Then we have
% \begin{align}
%     s_{i,1}+ s_{i,i} &= t_1(-q_1 + q_2) + t_2(q_1 + q_2) = q_1(t_2-t_1) + q_2(t_2+t_1)
% \end{align}
% Note that 
% \begin{align}
%     t_2 - t_1  &= \nonumber \\
%     t_2 + t_1 &= \nonumber 
% \end{align}
% Thus, we have 
% \begin{align}
%     s_{i,1}+ s_{i,i} &= q_1() + q_2() \nonumber \\
%     &= 
% \end{align}




    
% \end{proof}



% \begin{lemma}\label{lem:exp-w-quad}
    
% \end{lemma}

% \begin{proof}
    
% \end{proof}



% \begin{lemma}\label{lem:orthog}
    
% \end{lemma}

% \begin{proof}

% For any $i\in [n]\setminus \{j\}$,  we can write without loss of generality
% \begin{align}
%     u_i = c_1 u + c_2 \frac{U_\perp u_j}{\| U_\perp u_j \|_2} + c_3 z
% \end{align}
% where $z$ is some unit vector orthogonal to both $u$ and $U_\perp u_j$, and $c_1, c_2$ and $c_3$ satisfy $c_1^2 + c_2^2 + c_3^2  = 1$.





    
% \end{proof}
